# Supplementary material for: Variational formulation and monolithic solution of computational homogenization methods
Source: arXiv:2312.12771 source file (2023-12-20)
Supplement: Supplementary file 1 [file sec_appendix.tex]

Hallo Welt.
